# Supplementary material for: InsightEdit: Towards Better Instruction Following for Image Editing
Source: arXiv:2411.17323 source file (2024-11-26)
Supplement: Supplementary file 1 [file X_suppl.tex]

\clearpage
\setcounter{page}{1}
\maketitlesupplementary

% \section{Rationale}
% \label{sec:rationale}
% % 
% Having the supplementary compiled together with the main paper means that:
% % 
% \begin{itemize}
% \item The supplementary can back-reference sections of the main paper, for example, we can refer to \cref{sec:intro};
% \item The main paper can forward reference sub-sections within the supplementary explicitly (e.g. referring to a particular experiment); 
% \item When submitted to arXiv, the supplementary will already included at the end of the paper.
% \end{itemize}
% % 
% To split the supplementary pages from the main paper, you can use \href{https://support.apple.com/en-ca/guide/preview/prvw11793/mac#:~:text=Delete%20a%20page%20from%20a,or%20choose%20Edit%20%3E%20Delete).}{Preview (on macOS)}, \href{https://www.adobe.com/acrobat/how-to/delete-pages-from-pdf.html#:~:text=Choose%20%E2%80%9CTools%E2%80%9D%20%3E%20%E2%80%9COrganize,or%20pages%20from%20the%20file.}{Adobe Acrobat} (on all OSs), as well as \href{https://superuser.com/questions/517986/is-it-possible-to-delete-some-pages-of-a-pdf-document}{command line tools}.

\section{Supplementary Materials of Dataset}

\begin{figure*}[ht]    
    \centering    
    \includegraphics[width=0.8\linewidth]{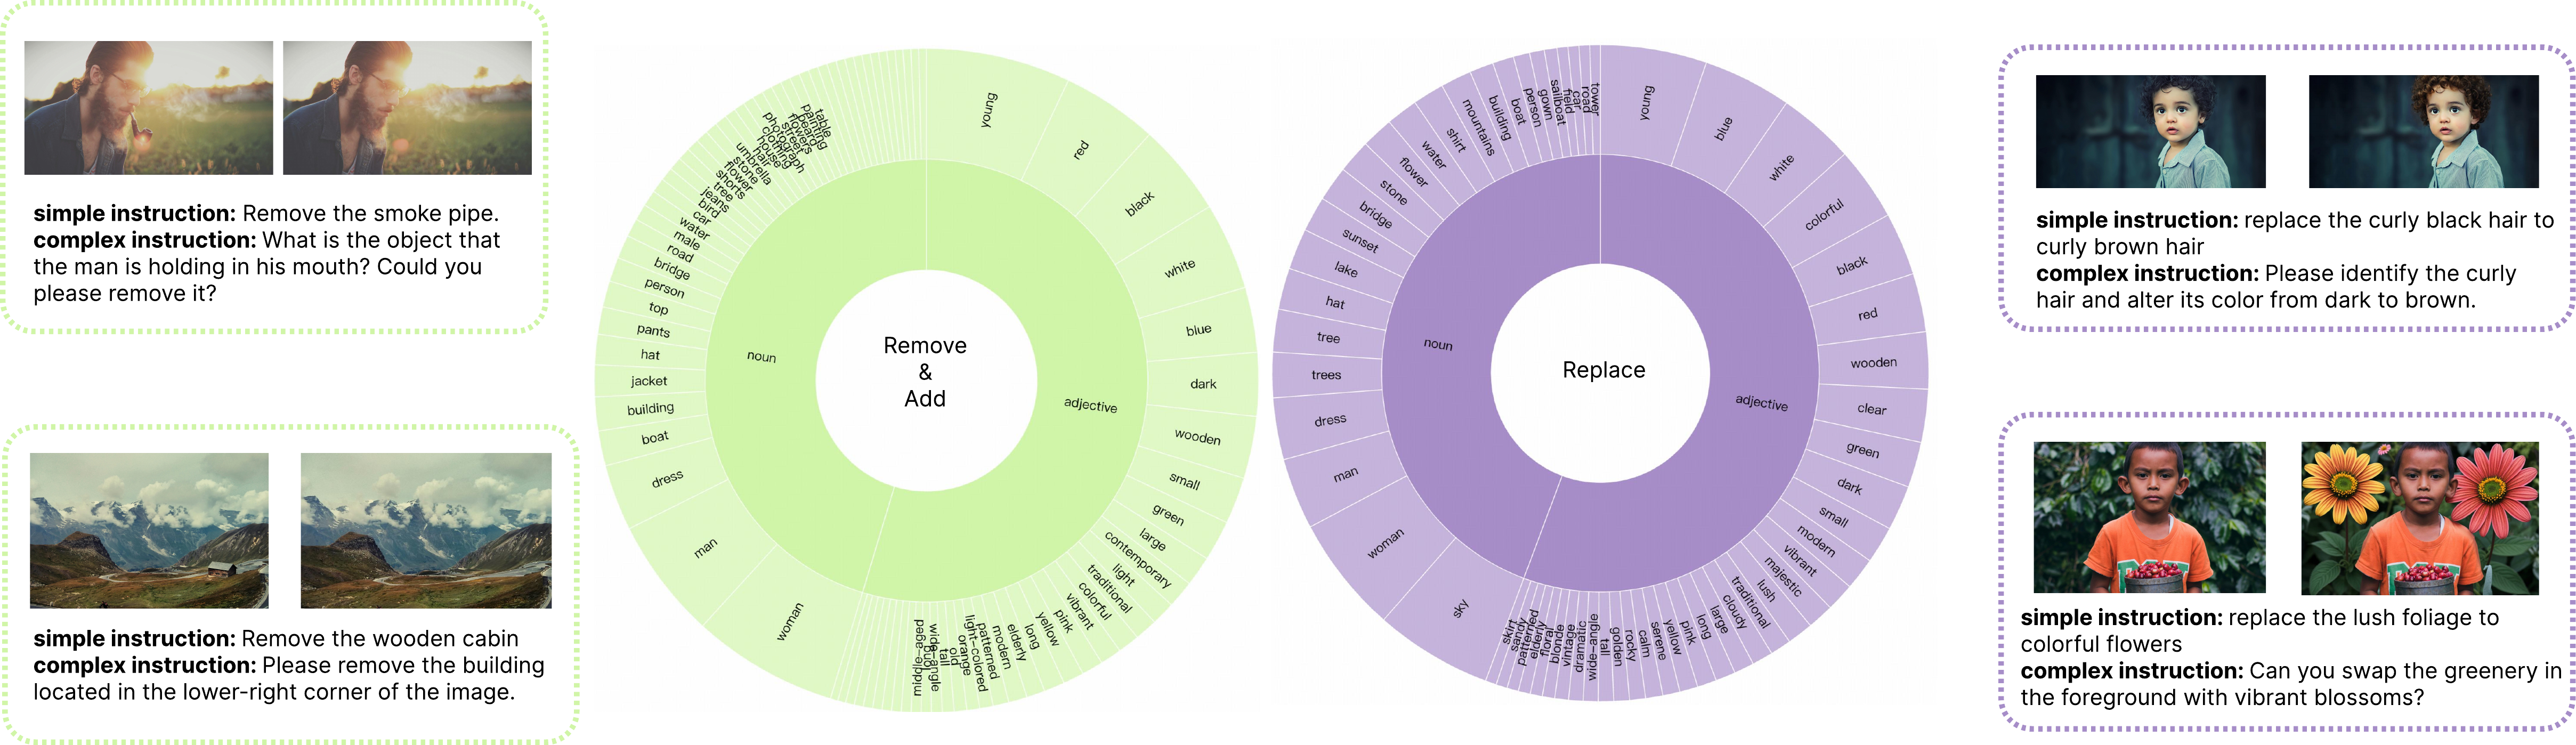}    
    \caption{Overall VisionEdit dataset. The left pie chart represents the object class keywords distribution in the addition and removal tasks, the right pie chart represents the object class keywords distribution in the replacement task. The cases on the left represents the removal image editing pairs with simple and complex instruction. The cases on the right represents the replacement image editing pairs with simple and complex instruction.}  
    \label{fig:dataset}    
\end{figure*}

\begin{figure}[htbp]
    \centering
    \includegraphics[width=0.5\textwidth]{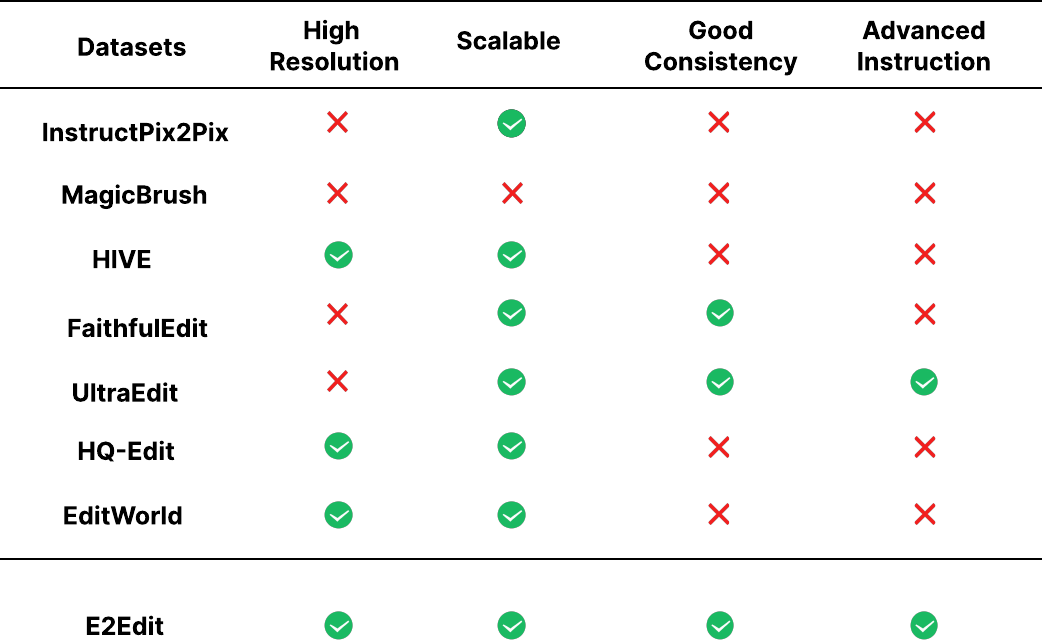} % 替换为你自己的图片文件路径
    \caption{Comparison with current dataset characteristics from four perspectives: resolution, scalability, consistency and instruction comple}
    \label{fig:dataset_comparison}
\end{figure}
\section{Supplementary Materials of Method}

\subsection{Training Stage1: Birdging VLM and SD}
The stage is to training bridging module which align hidden states of VLM into stable diffusion embedding space. We adopt two bridging strategy to extract both textual and visual information from hidden states. For the textual embedding, we apply Q-former to train learnable queries to align with the orginal clip text embedding of SD. For the visual embedding, a mapper in the CAM module is trained to align with the clip image embedding. The loss functions are as follow:
$$
\begin{aligned}
% & L_{\mathrm{LLM}}(c) = -\sum_{i=1}^r \log p_{\{\theta \cup \mathbf{E}\}}\left(\left[\mathrm{IMG}_i\right] \mid v_\mu(x), \right. \\
% & \left.s_1, \ldots, s_T, \left[\mathrm{IMG}_1\right], \ldots, \left[\mathrm{IMG}_{i-1}\right]\right) \\
& \mathbf{E}_{\text{text}} = \operatorname{CLIP}_{\text{text}}(\mathbf{t}) \\
& \mathbf{E}_{\text{image}} = \operatorname{CLIP}_{\text{image}}(\mathbf{I}_{\text{original}}) \\
& \operatorname{L}_{\text{text-feature}} = \frac{1}{N} \sum_{k=1}^N \left( \mathbf{E}_{\text{text}}^{(k)} - Q_\beta(h)^{(k)} \right)^2 \\
& \operatorname{L}_{\text{image-feature}} = \frac{1}{N} \sum_{k=1}^N \left( \mathbf{E}_{\text{image}}^{(k)} - \operatorname{Mapper}(h) \right)^2 \\
& \text{L}_{\text{stage1}} = \text{L}_{\text{LLM}} + \text{L}_{\text{text-feature}} + \text{L}_{\text{image-feature}} \\
\end{aligned}
$$
The loss function contains three loss function. The first is next token prediction loss of LLM(no vision encoder part in this stage). The second loss is the MSE loss between Qformer output embedding and the clip text encoder embedding. The third loss is the MSE loss between Mapper(a MLP layer in the CAM module) output embedding and the clip image encoder embedding.

\subsection{Training Stage2: Target Image Feature Acquisition}
% \begin{figure*}[ht]    
%     \centering    
%     \includegraphics[width=0.8\linewidth]{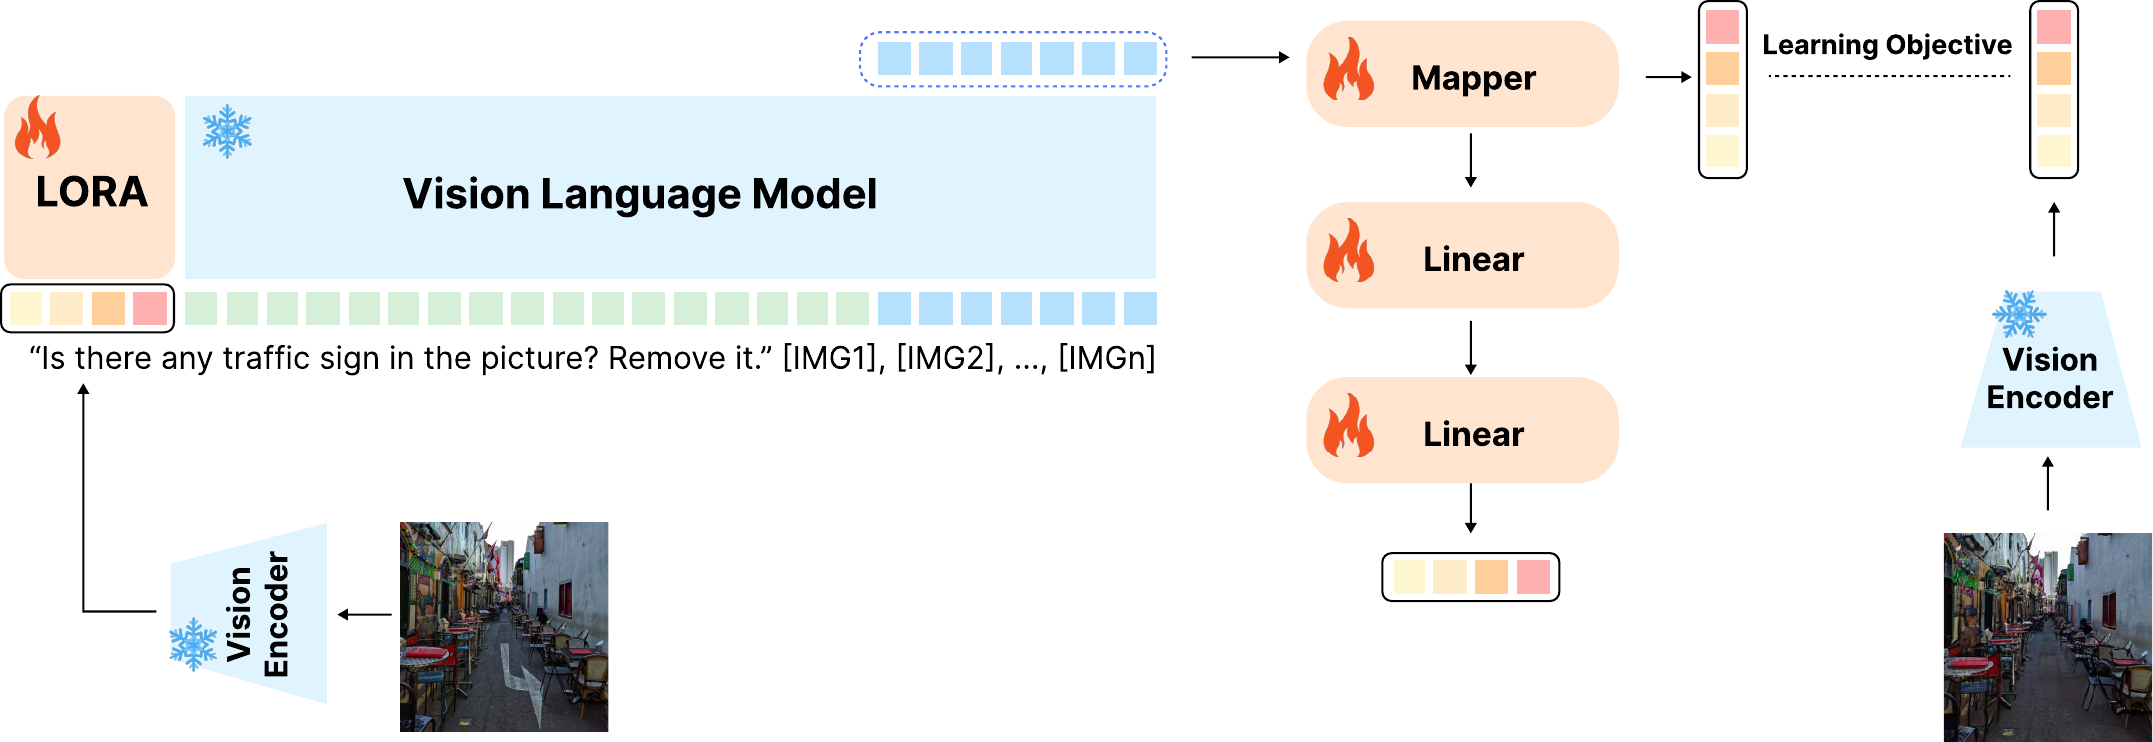}    
%     \caption{}  
%     \label{fig:training_detail}    
% \end{figure*}
In the training stage 2, we preliminarily train the capability that leverage the VLM to guide the SD's image editing. The trainable modules in this stage includes: the Lora module in VLM, the Q-former, the mapper layer in CAM module, the BIM module, the Unet. We add a explicit constraint in the CAM module, to let the visual embedding learn the feature of target image. The loss function is below:
$$
\begin{aligned}
& \mathbf{E}_{\text{image}} = \operatorname{CLIP}_{\text{image}}(\mathbf{I}_{\text{target}}) \\
& \operatorname{L}_{\text{target-image-feature}} = \frac{1}{N} \sum_{k=1}^N \left( \mathbf{E}_{\text{image}}^{(k)} - \operatorname{Mapper}(h) \right)^2 \\
& \text{L}_{\text{stage2}} = \text{L}_{\text{LLM}} + \text{L}_{\text{SD}} + \text{L}_{\text{target-image-feature}} \\
\end{aligned}
$$

\subsection{Training Stage3: Finetuning}
In the third training stage, we apply the de-coupled cross attention mechanism to exert both text and image features condition in image editing. The CAM module and the decouple cross attention in unet are the only trainable modules in this stage. The loss function of training stage 3 is as below:
$$
\begin{aligned}
\text{L}_{\text{stage3}} = \text{L}_{\text{target-image-feature}} + \text{L}_{\text{SD}}
\end{aligned}
$$

\begin{figure*}[ht]    
    \centering    
    \includegraphics[width=0.8\linewidth]{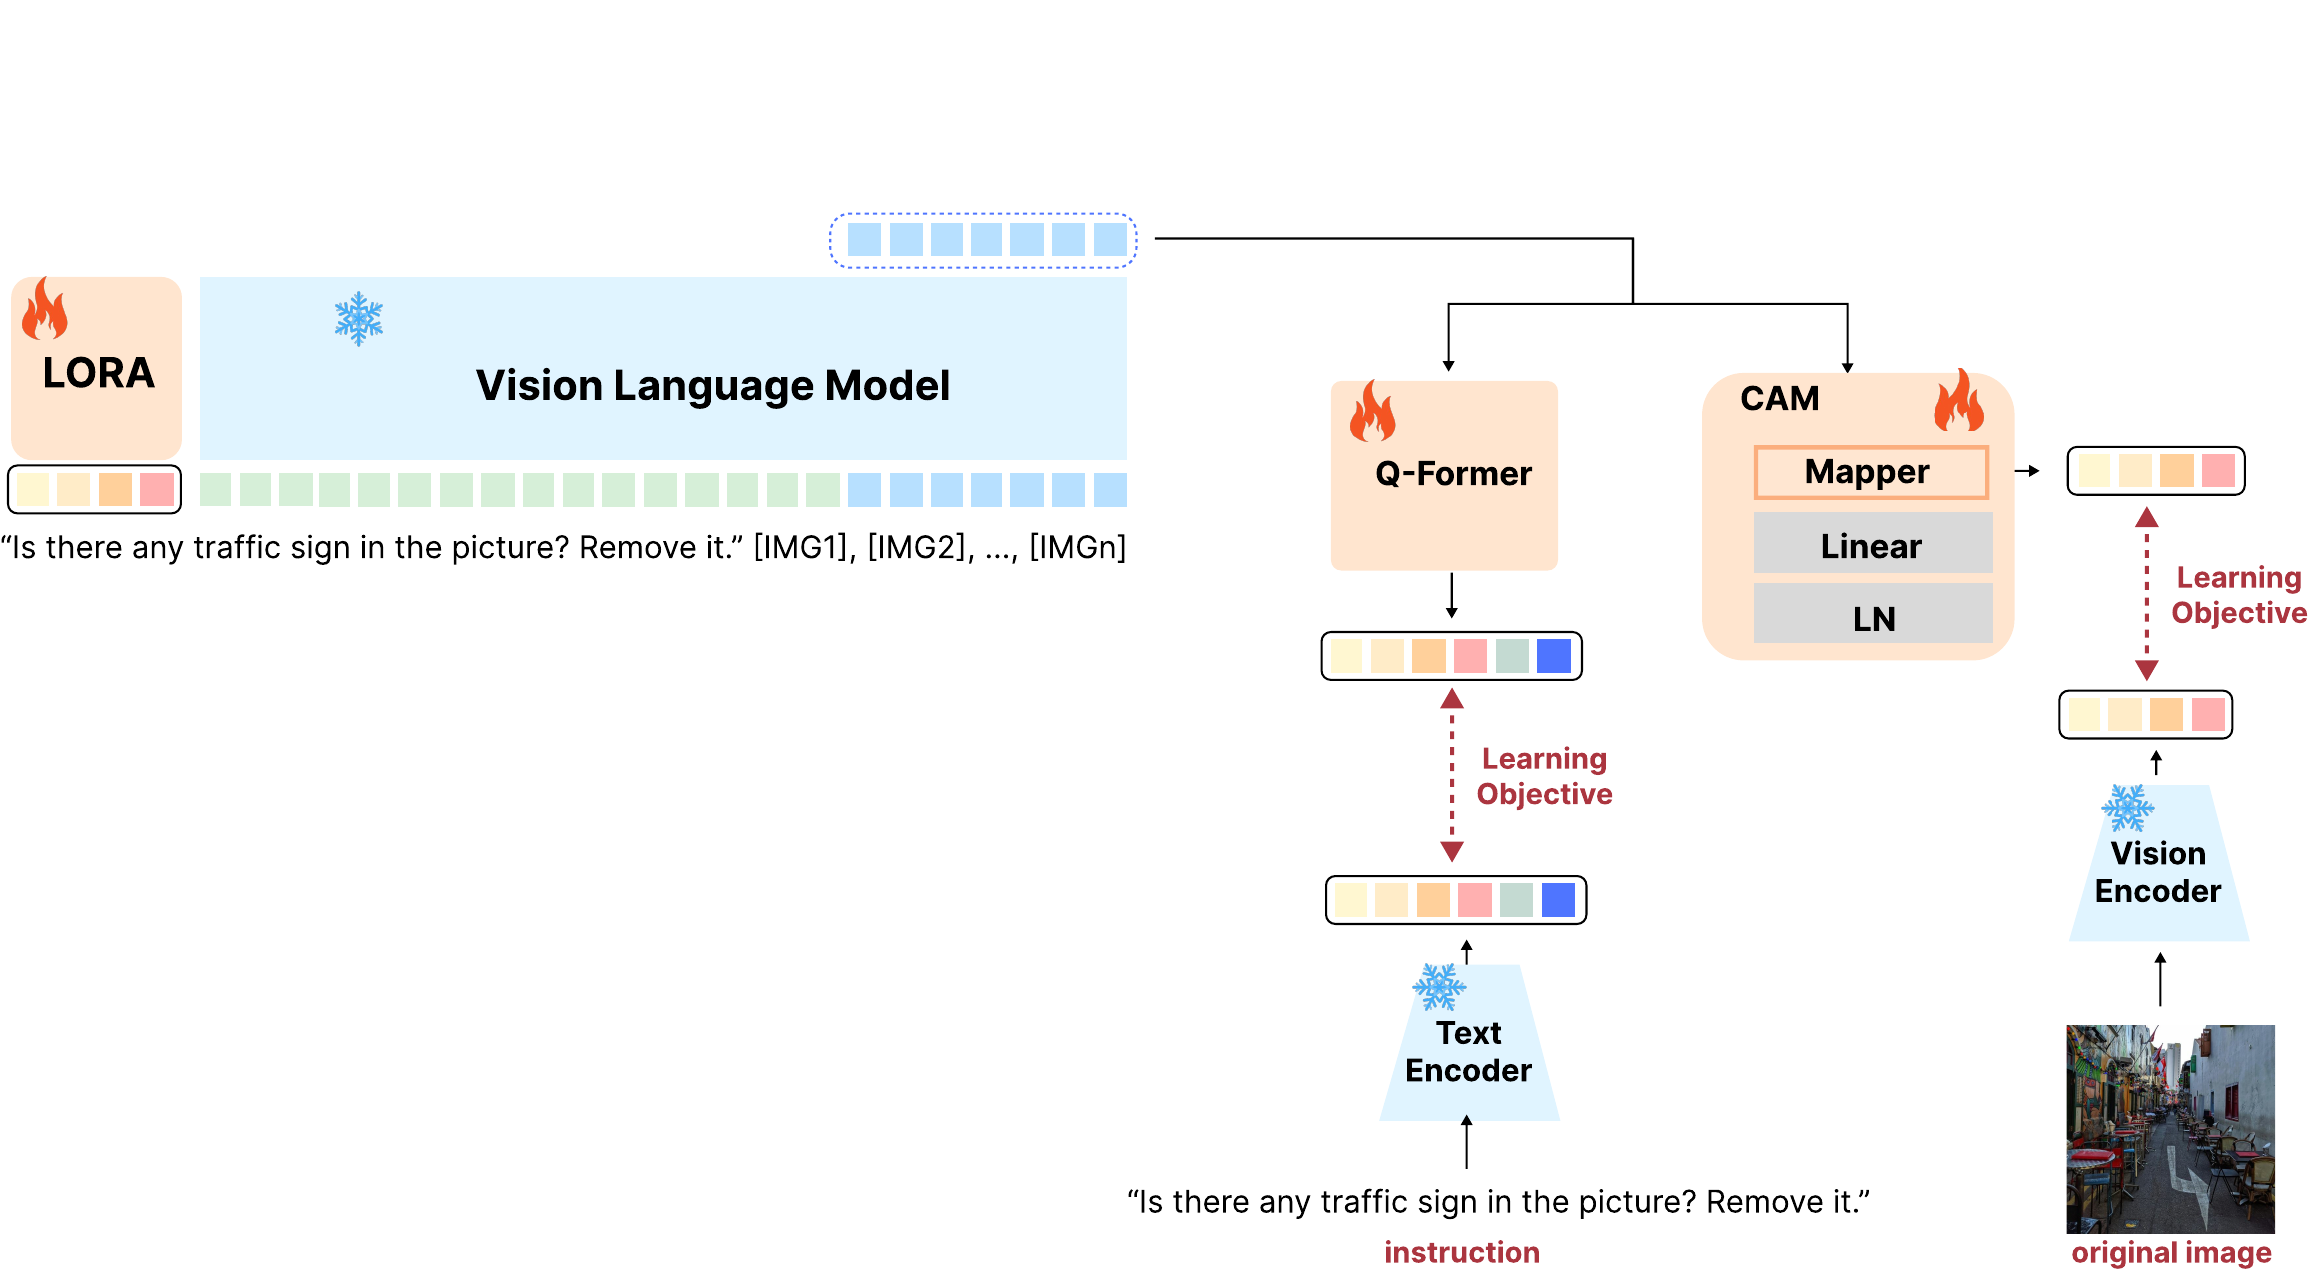}    
    \caption{}  
    \label{fig:training_stage1}    
\end{figure*}

\begin{figure*}[ht]    
    \centering    
    \includegraphics[width=0.8\linewidth]{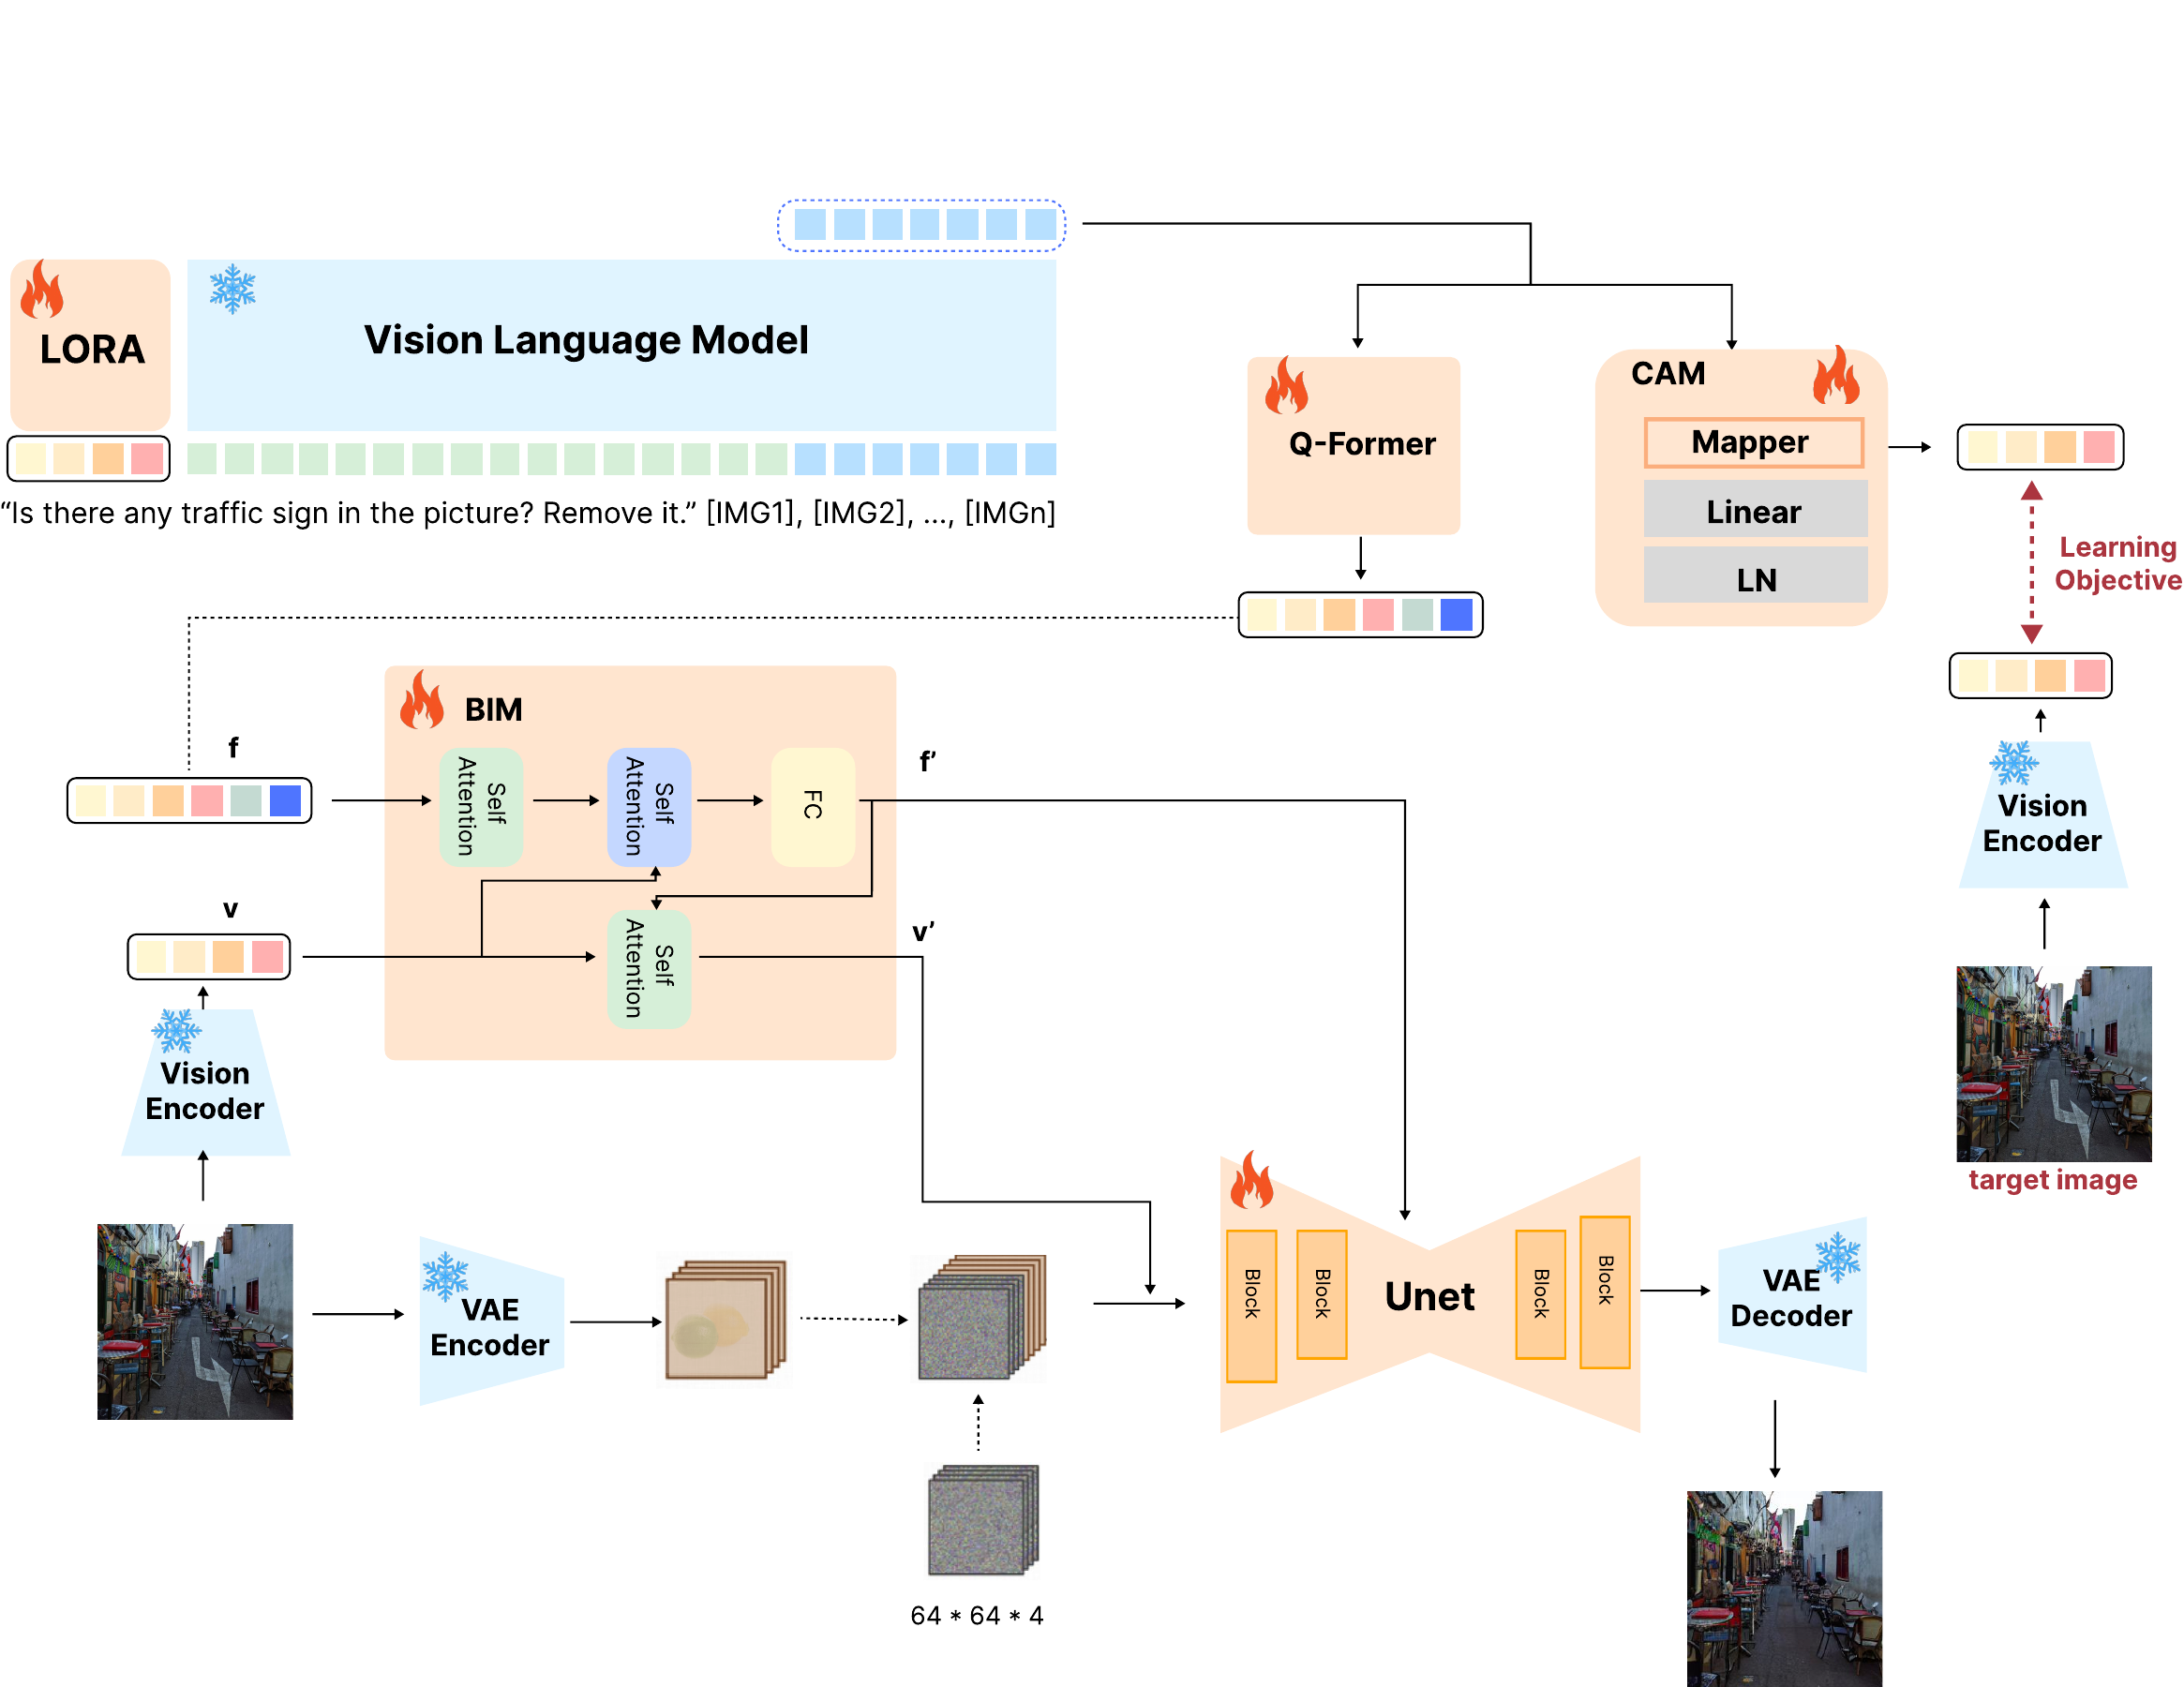}    
    \caption{}  
    \label{fig:training_stage2}    
\end{figure*}

\begin{figure*}[ht]    
    \centering    
    \includegraphics[width=0.8\linewidth]{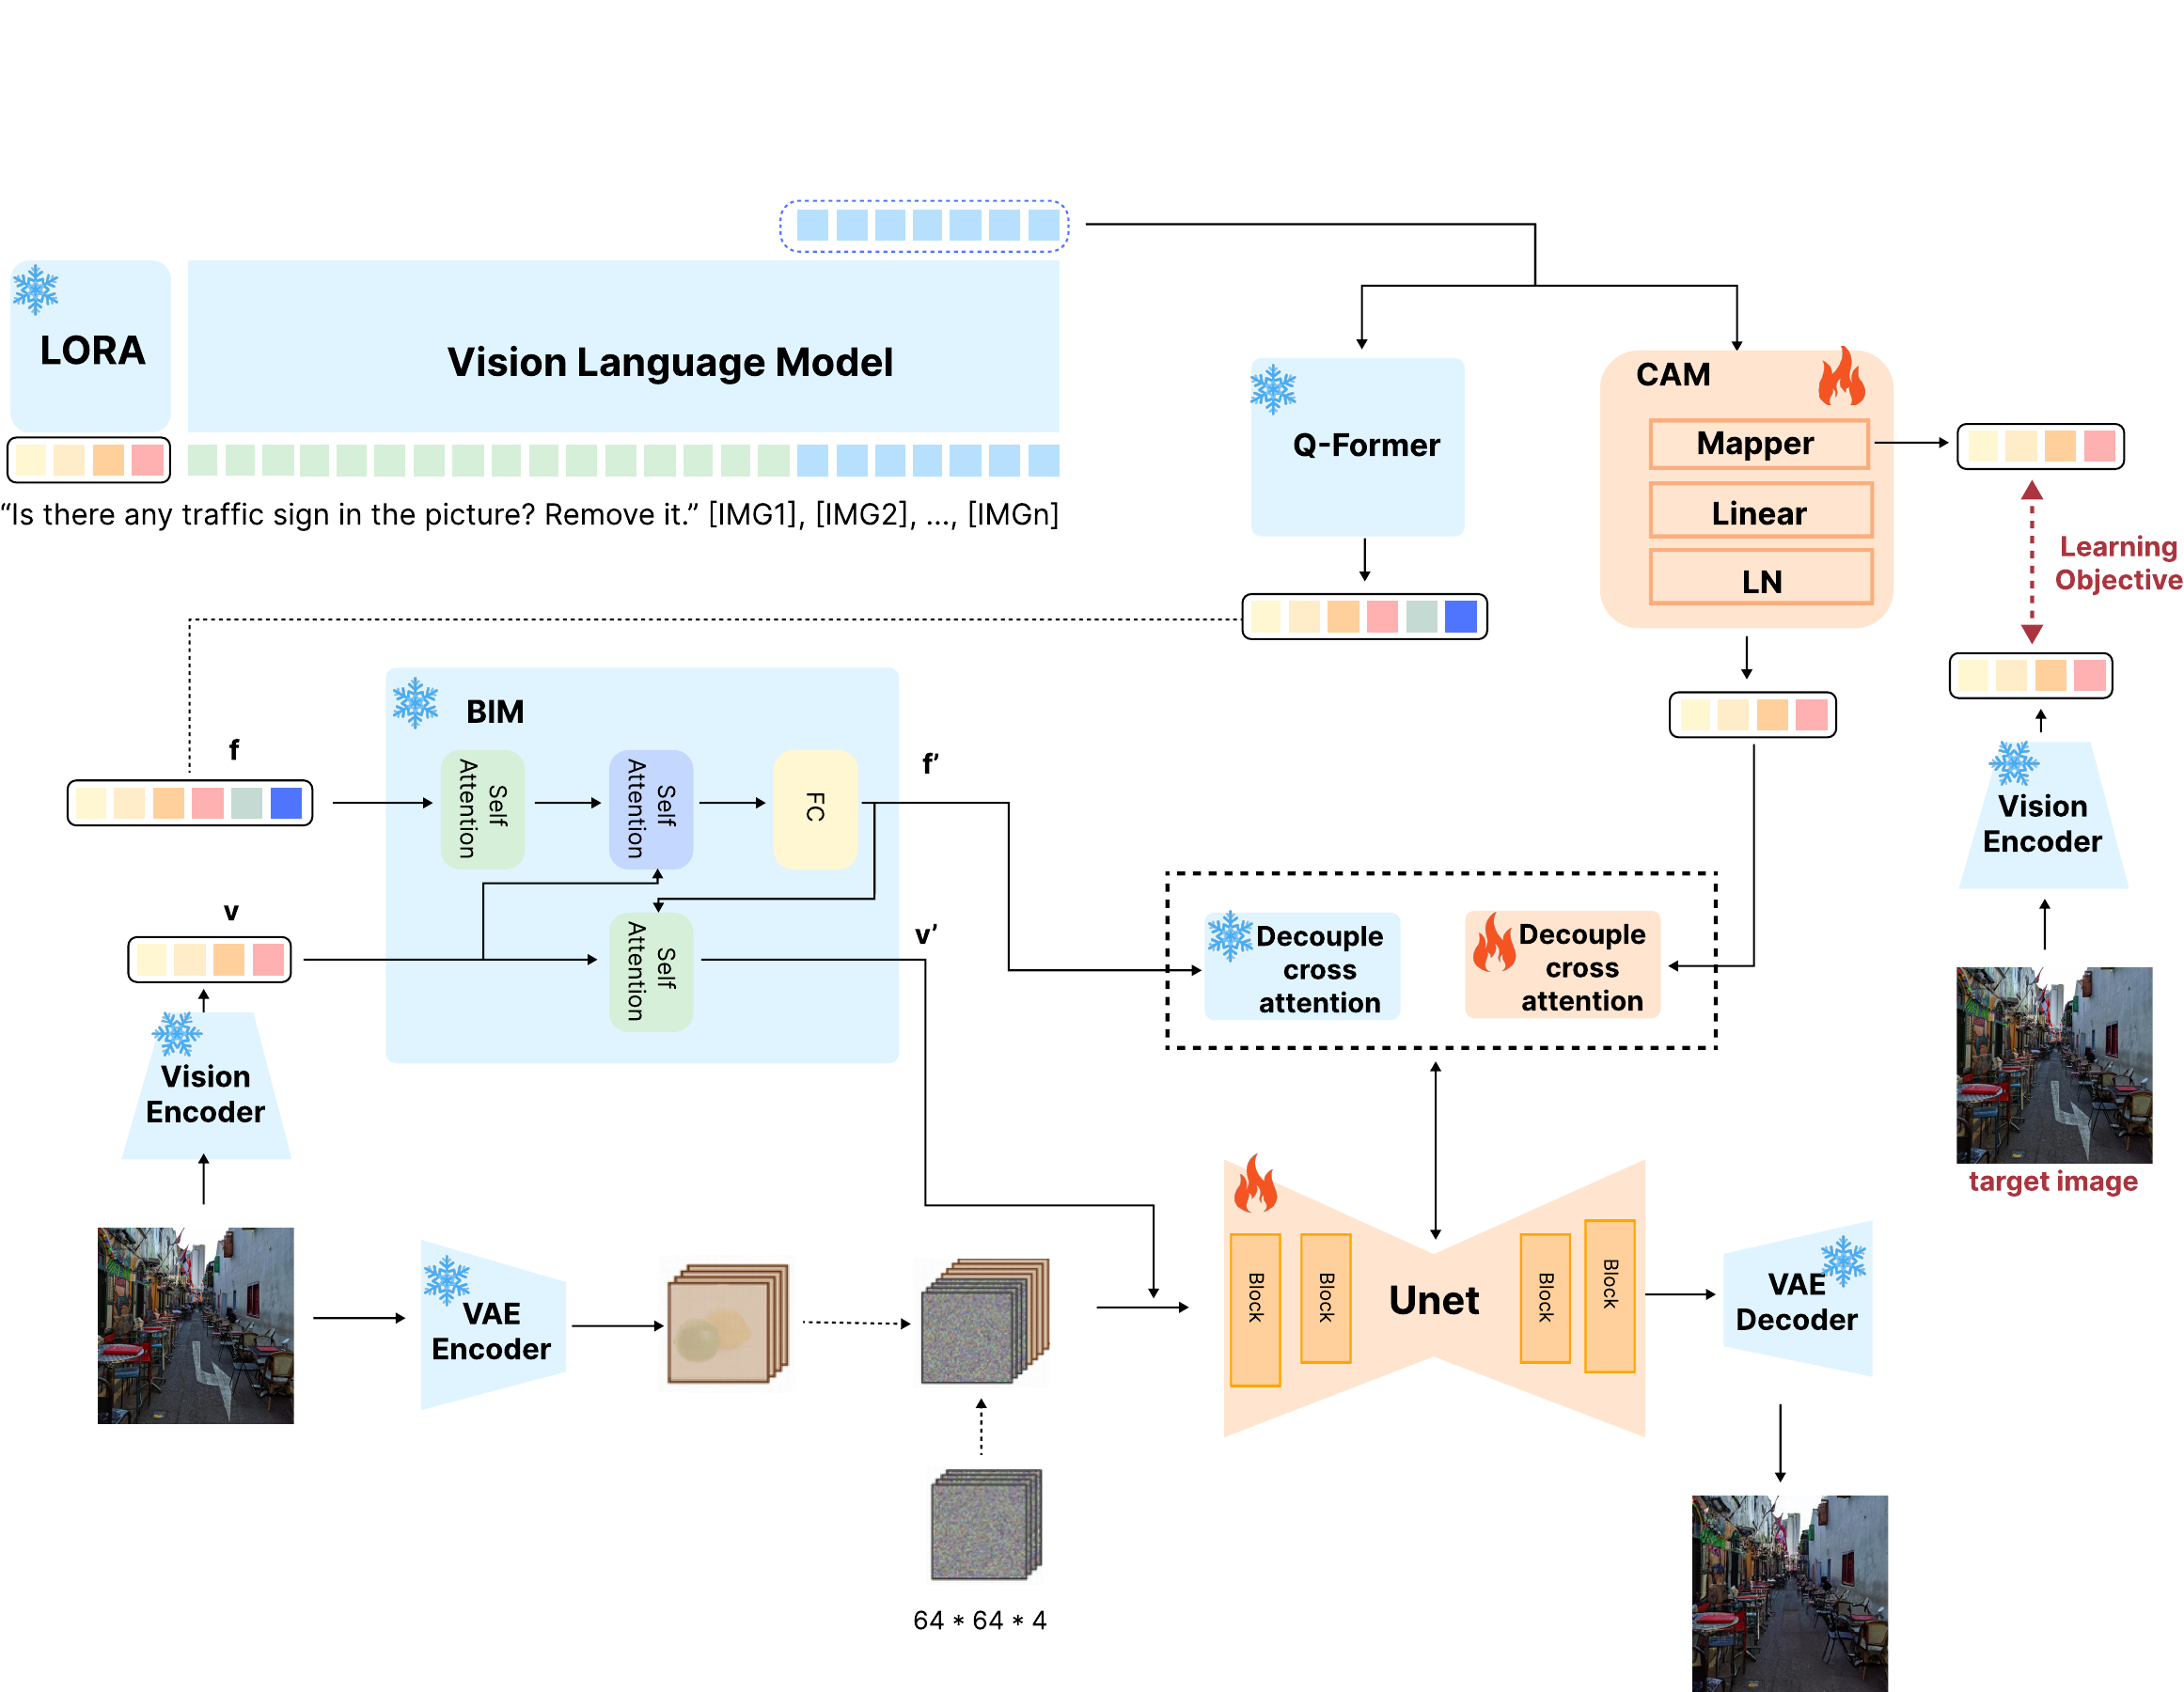}    
    \caption{}  
    \label{fig:training_stage3}    
\end{figure*}

\subsection{Comprehension and Generation in Image Editing}
Increasingly, researchers are exploring the unification of understanding and generation in computer vision. GILL\cite{koh2024generating} is the first to employ a mapper that aligns the understanding embeddings of VLM with the generation embeddings of SD. MoMa\cite{song2024moma} further integrates visual concepts with text prompts to facilitate personalized image generation. Other works, such as Transfusion\cite{zhou2024transfusion}, DreamLLM\cite{dong2023dreamllm}, have also investigated unified architectures. In the context of image editing tasks, MGIE\cite{fu2023guiding} replaces the existing CLIP text encoder with LLaVA\cite{liu2024visual}, endowing the model with the ability to comprehend complex instructions. SmartEdit\cite{huang2024smartedit} intrudes a BIM module that enables comprehensive bidirectional information interation between the image and the LLM output.

% 构造数据中的掩码调试和背景保持，影响数据构造的整体质量
It is noteworthy that two key factors significantly influence the overall quality of the generated images. The first factor is the closing operation applied to the masks. Since mask-based models typically rely on manual brushing operations, there are noticeable differences in the image patterns compared to those generated by segmentation models. Therefore, we need to employ a closing operation on the original mask to smooth the edges of the segmentation and fill any gaps within the masked regions. Another important aspect is the use of blending operations to ensure consistency between the unmodified areas and the original image.
